# Supplementary material for: Movable Dirac Points with Ferroelectrics: Kink States and Berry Curvature Dipoles
Source: arXiv:2506.13960 source file (2025-06-16)
Supplement: Supplementary file 1 [file KS_Supplemental_Material.pdf]

# Supplemental Material

# Movable Dirac Points with Ferroelectrics: Kink States and Berry Curvature Dipoles

Konstantin S. Denisov[1], Yuntian Liu[1], and Igor Žutić[1]

[1] *Department of Physics, University at Buffalo, State University of New York, Buffalo, NY 14260, USA*

Contents: Notes I-IV, Table S1, Figures S1,S2

## Note I. Materials Hosting Movable Dirac Points

Table S1. Material candidates with movable Dirac points (DPs). The materials are selected from Topological 2D Materials Database [1,2]. We also provide the corresponding layer group symbols and the position of the movable DPs, by indetifying the high-symmetry line and the corresponding high-symmetry point.

| Materials | Layer Group | Position of DPs |
|---|---|---|
| $Mo_2S_4$ | 15 | Γ-Y (near Γ) |
| $W_2Se_4$ | 15 | Γ-Y (near Γ) |
| $As_2F_2$ | 15 | S-X (near X) |
| $Bi_2Br_2$ | 15 | S-X (near X) |
| $Br_2Sb_2$ | 15 | S-X (near X) |
| $F_2P_2$ | 15 | S-X (near X) |
| $Ir_2Nb_2Te_8$ | 15 | S-X (near X) |
| $Mo_2Se_4$ | 15 | Γ-Y (near Γ) |
| $Nb_2Rh_2Te_8$ | 15 | S-X (near X) |
| $Cu_4I_8$ | 16 | Γ-X (near X) |
| $Hg_8O_4$ | 17 | Γ-Y (near Y) |
| $Hg_4N_4S_4$ | 17 | Γ-X (near X) |
| $Hg_{10}O_4$ | 17 | Γ-Y (near Y) |

| | | |
|---|---|---|
| $Hg_3S_2$ | 18 | Γ-Y (near Y) |
| $As_2Br_2$ | 18 | Γ-Y (near Y) |
| $I_2Re_2$ | 18 | Γ-Y (mid) |
| $I_2Sb_2$ | 18 | Γ-Y (near Y) |
| $Se_8Sn_2Ta_4$ | 44 | Γ-X (near Γ) |
| $I_2N_2Ti_2$ | 46 | Γ-X (near Γ) |
| $Br_2Rh_2S_2$ | 46 | Γ-Y (near Γ) |
| $Cl_2Rh_2S_2$ | 46 | Γ-Y (near Γ) |
| $Co_2F_2O_2$ | 46 | Γ-Y (near Γ) |
| $F_2Rh_2S_2$ | 46 | Γ-Y (near Γ) |
| $Hf_2Se_{10}$ | 46 | Γ-X (near Γ) |
| $I_2N_2Ti_2$ | 46 | Γ-Y (near Γ) |
| $S_{10}Zr_2$ | 46 | Γ-X (near Γ) |
| $Se_{10}Zr_2$ | 46 | Γ-X (near Γ) |
| $Te_{10}Zr_2$ | 46 | Γ-X (near Γ) |
| $P_2Rh_2Se_6$ | 71 | Γ-K; Γ-M (near Γ) |
| $Hf_2S_2$ | 72 | Γ-K (mid) |
| $S_2Ti_2$ | 72 | Γ-K (mid) |
| $S_2Zr_2$ | 72 | Γ-K (mid) |
| $Se_2Ti_2$ | 72 | Γ-K (mid) |
| $Se_2Zr_2$ | 72 | Γ-K (mid) |
| $Te_2Ti_2$ | 72 | Γ-K (mid) |
| $Te_2Zr_2$ | 72 | Γ-K (mid) |

**Note II. First-Principles Calculations**

Our first-principles calculations were conducted using the Vienna ab initio simulation package (VASP) [3] that employed the projector augmented wave [4] method within the framework of density-functional theory [5,6]. The exchange-correlation functional was described through the generalized gradient approximation

with the Perdew-Burke-Ernzerhof formalism [7,8]. The plane-wave cutoff energy was set to 500 eV and the van der Waals correction was included via the DFT-D3 [9]. The force and total energy convergence criteria were set to 0.005 eV/Å and $1.0\times10^{-6}$ eV, respectively. Sampling of the entire Brillouin zone was performed by a $11\times13\times1$ Monkhorst-Pack grid. The Berry curvature was calculated from a tight-binding Hamiltonian based on the Wannier functions [10,11] and WannierTools package [12], using the Kubo formula [13,14]:

$$\Omega_n^z(\boldsymbol{k}) = \sum_{n'\neq n} \frac{2Im\left[\langle \boldsymbol{k}n|\hat{v}_x|\boldsymbol{k}n'\rangle\langle \boldsymbol{k}n'|\hat{v}_y|\boldsymbol{k}n\rangle\right]}{(\epsilon_{\boldsymbol{k}n}-\epsilon_{\boldsymbol{k}n'})^2}$$

$$\Omega^z(\boldsymbol{k}) = \textstyle\sum_n f_{\boldsymbol{k}n}\,\Omega_n^z(\boldsymbol{k})$$

$$\Omega^z(k_y) = \int_0^{2\pi/a}\Omega^z(\boldsymbol{k})dk_x \qquad \text{(S1)}$$

where $|\boldsymbol{k}n\rangle$ and $\epsilon_{\boldsymbol{k}n}$ are the eigenstate and eigenvalue for band $n$ with wave vector $\boldsymbol{k}$. $\hat{v}_i$ $(i = x, y)$ is velocity operator along the $i$ direction. $a$ is the lattice constant.

**Note III. Crystal and Band Structures of the $Cl_2Rh_2S_2$-GeS Junction and the Impact of Spin-Orbit Coupling**

To illustrate the details of the $Cl_2Rh_2S_2$-GeS junction, we present the complete crystal structures for both FE1 and FE2 states, as well as the global band structures for these states without and with SOC. The optimized lattice constants of $Cl_2Rh_2S_2$-GeS junction are $a$ = 4.63 Å and $b$ =3.52 Å. As shown in Fig. S1(a-b), the FE polarization of GeS is oriented along the $a$-axis, perpendicular to the $\Gamma$-$Y$ path containing the movable Dirac points. The FE switching of GeS causes changes in interlayer stacking but has minimal impact on the band structure. Figures S1(c)-S1(d) indicate that both FE1 and FE2 states open an energy gap at the Dirac points, with $E_g = 33.3\,meV$ for FE1 and $E_g = 18.0\,meV$ for FE2. Calculations including the spin-orbit coupling (SOC) show that it has a negligible impact on the band structure, illustrating the robustness of both FE states under SOC.

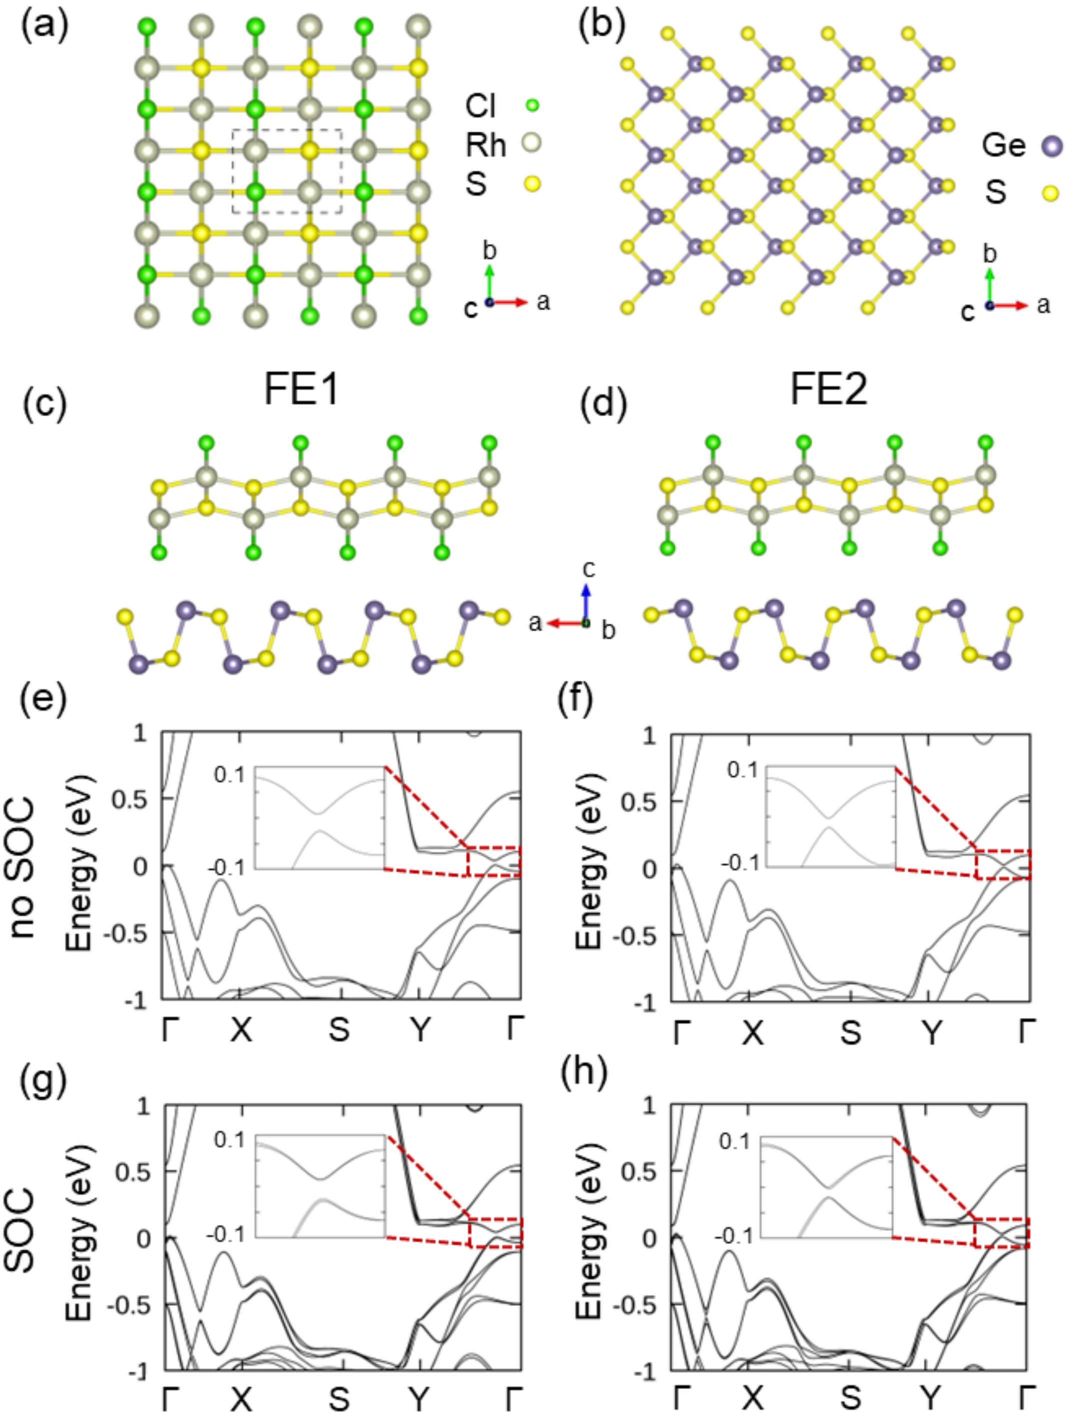


Fig. S1. (a) Top view of the crystal structures of $Cl_2Rh_2S_2$. (b) Top view of the crystal structures of GeS. (c), (d) Side view of the crystal structures of the $Cl_2Rh_2S_2$-GeS junction in the (c) FE1 state and (d) FE2 state. (e), (f) Band structures of the $Cl_2Rh_2S_2$-GeS junction in the (c) FE1 state and (d) FE2 state without SOC. (g), (h) Band structures of the $Cl_2Rh_2S_2$-GeS junction in the (g) FE1 state and (h) FE2 state with SOC. The insets show the magnified band structures near the gapped Dirac points.

**Note IV. Tight-Binding Model of Movable Dirac Points**

The considered spinless lattice tight-binding (TB) model is shown in Fig. S2. It consists of the two oppositely oriented zigzag chains (indicated by solid and dashed lines connecting neighboring sites) coupled to each other with an on-site coupling constant, $\gamma$, the geometry of the lattice is also shown in Fig. S2. Each zigzag chain has two inequivalent sites connected by a nearest neighbor hopping parameter, $t/2$. In the absence of the interchain coupling, $\gamma = 0$, the nearest neighbor TB Hamiltonian of each chain is a 2x2 matrix (in the basis of 2 inequivalent sites) in k-space given by

$$H_{1c}(k_x, k_y) = \begin{pmatrix} 0 & -t\cos(k_x a_0/2)e^{\mp i k_y b_0/2} \\ -t\cos(k_x a_0/2)e^{\pm i k_y b_0/2} & 0 \end{pmatrix}, \quad (S2)$$

where $\pm$ reflects the geometrical orientation of sites within each chain. Using the notation from the main text, we introduce $h = h_x + i h_y = \cos(k_x a_0/2)e^{i k_y b_0/2}$, allowing us to present $H_{1c}(k_x, k_y) = -t(h_x\sigma_x \pm h_y\sigma_y)$, where the Pauli $\sigma$ matrices are related to inequivalent sites within one chain. The sign factor in the second term can be modelled by the Pauli matrix, $\tau_z$, accounting for the chain index. With Pauli matrices, $\sigma$ and $\tau$, the inclusion of the finite interchain hybridization, $\gamma$, in the geometry of Fig. S2, will be described in the 4x4 Hamiltonian by the term, $-\gamma\tau_x$. Furthermore, we also introduce the on-site staggered potential, $u$, which has the opposite sign for two inequivalent sites within the same chain, requiring $\sigma_z$, (this makes the effective Hamiltonian of each chain match the Su-Schrieffer-Heeger model [15]) and for two different chains, see Fig. S2, also requiring $\tau_z$. The resulting staggered chain-dependent on-site potential has the form, $u\sigma_z\tau_z$. Figures S2(a) and S2(b) show the high-symmetry ($u = 0$) and low-symmetry ($u \neq 0$) lattice configurations featuring gapless (a) and gapped (b) Dirac points along the $\Gamma - X$ line.

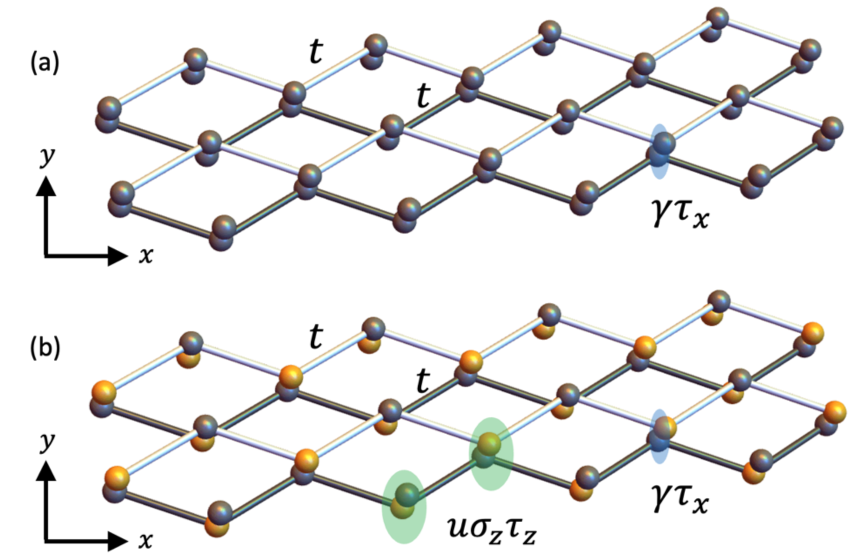


Fig. S2. (a) High- and (b) low-symmetry lattice configuration used for the tight-binding model of 2D movable Dirac points.

**Note V. Motion of Dirac Points by Deformation**

In this section we provide the analysis for the band structure transformation of a monolayer $Cl_2Rh_2S_2$ at a finite deformation.

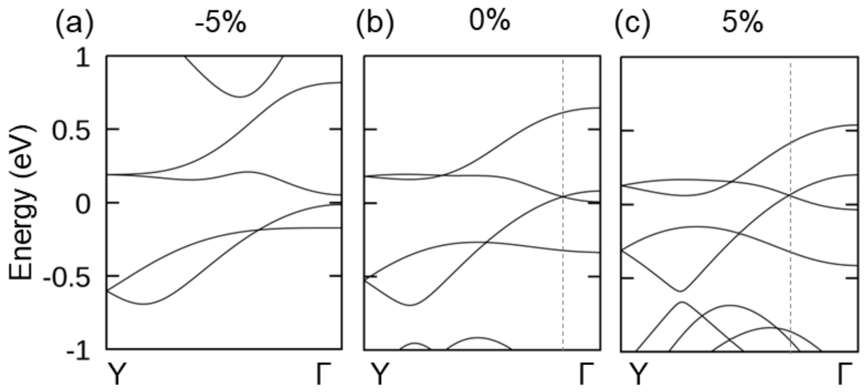


Fig. S3. Band structures along the Y-Γ line of $Cl_2Rh_2S_2$ under different strains. (a) 5% compression along the a-axis. (b) No strain. (c) 5% tension along the a-axis. The positions of the Dirac points near the Fermi level are marked by gray dashed lines in panels (b) and (c).

Table S2. Positions of the Dirac points under different strains. The a axis and b axis in the first column indicate the crystal directions along which strain is applied. The position of each Dirac point is given as a ratio of its distance from the Γ point to the total Γ–Y path length.

| Strain | -5.0% | -2.5% | 0 | +2.5% | +5% |
|---|---|---|---|---|---|
| a axis | -- | 0.00 | 0.16 | 0.24 | 0.29 |
| b axis | 0.18 | 0.18 | 0.16 | 0.14 | 0.11 |

## References


[1] U. Petralanda, Y. Jiang, B. A. Bernevig, N. Regnault, and L. Elcoro, *Two-dimensional Topological Quantum Chemistry and Catalog of Topological Materials*, arXiv:2411.08950v1 (2024).

[2] Y. Jiang, U. S. Petralanda, G. , Q. Xu, H. Pi, D. Călugăru, H. Hu, J. Xie, R. A. Mustaf, P. Höhn, V. Haase *et al.*, *2D Theoretically Twistable Material Databas*, arXiv:2411.09741v1 (2024).

[3] G. Kresse, and J. Furthmuller, *Efficient iterative schemes for ab initio total-energy calculations using a plane-wave basis set*, Phys. Rev. B **54**, 11169 (1996).

[4] G. Kresse, and D. Joubert, *From ultrasoft pseudopotentials to the projector augmented-wave method*, Phys. Rev. B **59**, 1758 (1999).

[5] P. Hohenberg, and W. Kohn, *Inhomogeneous electron gas*, Phys. Rev. **136**, B864 (1964).

[6] W. Kohn, and L. J. Sham, *Self-Consistent Equations Including Exchange and Correlation Effects*, Phys. Rev. **140**, 1133 (1965).

[7] J. P. Perdew, K. Burke, and M. Ernzerhof, *Generalized Gradient Approximation Made Simple*, Phys. Rev. Lett. **77**, 3865 (1996).

[8] J. P. Perdew, K. Burke, and M. Ernzerhof, *Generalized Gradient Approximation Made Simple,* Phys. Rev. Lett. **78**, 1396 (1997).

[9] S. Grimme, J. Antony, S. Ehrlich, and H. Krieg, *A consistent and accurate ab initio parametrization of density functional dispersion correction (DFT-D) for the 94 elements H-Pu*, J. Chem. Phys. **132**, 154104 (2010).

[10] A. A. Mostofi, J. R. Yates, Y. S. Lee, I. Souza, D. Vanderbilt, and N. Marzari, *wannier90: A tool for obtaining maximally-localised Wannier functions*, Comput. Phys. Commun. **178**, 685 (2008).

[11] N. Marzari, A. A. Mostofi, J. R. Yates, I. Souza, and D. Vanderbilt, *Maximally localized Wannier functions: Theory and applications*, Rev. Mod. Phys. **84**, 1419 (2012).

[12] Q. S. Wu, S. N. Zhang, H. F. Song, M. Troyer, and A. A. Soluyanov, *WannierTools: An open-source software package for novel topological materials*, Comput. Phys. Commun. **224**, 405 (2018).
[13] D. J. Thouless, M. Kohmoto, M. P. Nightingale, and M. den Nijs, *Quantized Hall Conductance in a Two-Dimensional Periodic Potential*, Phys. Rev. Lett. **49**, 405 (1982).
[14] D. Xiao, M. C. Chang, and Q. Niu, *Berry phase effects on electronic properties*, Rev. Mod. Phys. **82**, 1959 (2010).
[15] W.-P. Su, J. R. Schrieffer, and A. J. Heeger, *Solitons in Polyacetylene,* Phys. Rev. Lett. 42, 1698 (1979).
